# Supplementary material for: Nonlocal pseudopotentials and time-step errors in diffusion Monte Carlo
Source: arXiv:2104.00797 ancillary file (2021-07-27)
Supplement: Supplementary file 1 [file suppl.pdf]

# Supplementary Material for
# Nonlocal pseudopotentials and time-step errors in diffusion Monte Carlo

Tyler A. Anderson [a] and C. J. Umrigar [b]
*Laboratory of Atomic and Solid State Physics,*
*Cornell University, Ithaca, NY 14853.*

[a] taa65@cornell.edu
[b] CyrusUmrigar@cornell.edu

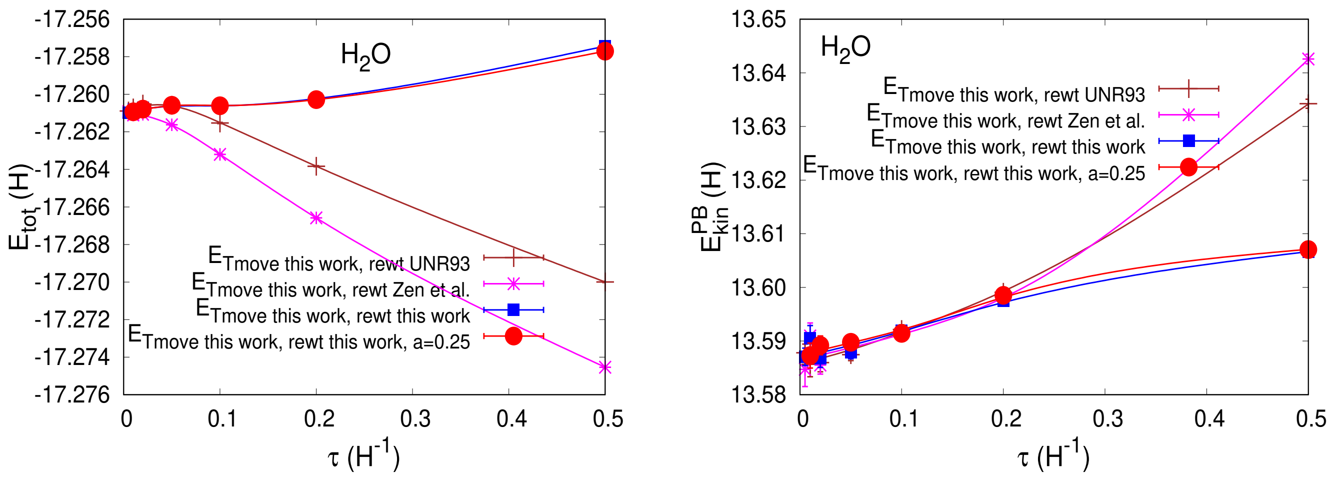


(a) (b)

FIG. 1. Time step error of the total energy (a) and of the kinetic energy (b) of $H_2O$, demonstrating the effect of the average drift velocity parameter, $a$, and of the various reweighting factors. All the curves use the T-moves algorithm of this paper, and are least squares quadratic fits.

In Fig. 1 we address two issues that were glossed over in the main text, using $H_2O$ as an example. First, we show that the dependence on the parameter $a$ appearing in the average drift velocity is fairly weak, by comparing the time-step errors for $a = 0.5$ and $a = 0.25$. Second, in the main text we showed that the reweighting factor of Eq. 9 of the main text results in a smaller time-step error in the total energy than the reweighting factors of Refs. 7 and 8 when using the locality approximation. Fig. 1 shows that the same is true when using the T-moves approximation of this paper.

In the main text we observed that the Casula et al. T-moves results in a very large time-step dependence of the kinetic energy for all the systems studied except $Si_{15}$. The likely reason for this is that the silicon pseudopotential is not as nonlocal as the carbon and oxygen pseudopotentials. In Fig. 2 we plot the Burkatzki-Filippi-Dolg (BFD) pseudopotentials[1] for these three atoms. At $r = 0$, the s and the p pseudpotentials for carbon and oxygen differ by 23 and 38 Ha respectively, whereas those for silicon differ by only 6 Ha. Note that, for silicon, the d pseudopotential differs considerably from the s and p pseudpotentials but this is of little importance because only s and p orbitals are occupied in silicon.

In Table I we provide the VMC energies for each system to indicate the quality of the trial wave functions used.

TABLE I. VMC energies for each system.

| System | Energy (Ha) |
|---|---|
| C, 1 CSF | $-5.416054(7)$ |
| C, 29 CSFs | $-5.43221(1)$ |
| Cr | $-86.7258(2)$ |
| $H_2O$ | $-17.24794(4)$ |
| Butadiene | $-26.27055(7)$ |
| $Si_{15}$ | $-58.3764(6)$ |

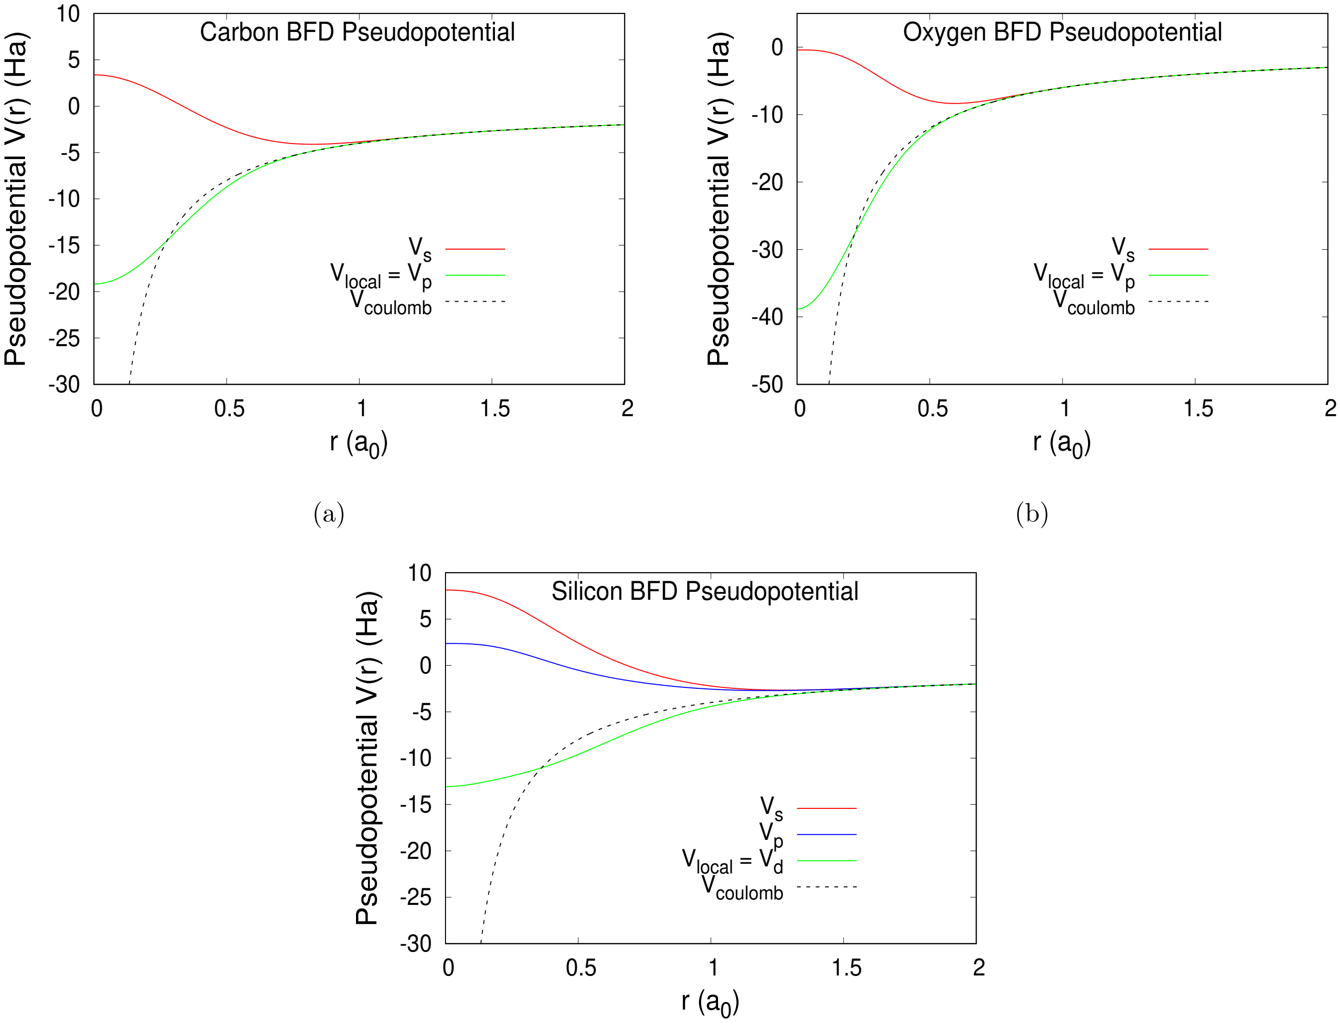


(a) (b) (c)

FIG. 2. Burkatzki-Filippi-Dolg (BFD) pseudopotentials for carbon, oxygen, and silicon used in this work.

[1] M. Burkatzki, C. Filippi, and M. Dolg, J. Chem. Phys. **129**, 164115 (2008).
